# Supplementary material for: Dash: Scalable Hashing on Persistent Memory
Source: arXiv:2003.07302 source file (2020-04-09)
Supplement: Supplementary file 1 [file appendix.tex]

\appendix
In this appendix we present detailed algorithms for insert, delete and search operations, as well as the recovery process in DASH.
\section{DASH-EX Operations}

\label{sec:ops}
\subsection{Insert}
New records are added to the free space available in the bucket.
To insert a record $r$, a thread first check the version lock on the directory.
If the lock is set, this means there is an on-going directory modification, 
in this case the current thread must wait until the structure modification finishes.
Otherwise, the thread will compute the hash value $h$ of the key and use it to locate the corresponding bucket $b$ and its neighbor bucket $b+1$.
This is done by using the least $n$ bits of $h$ to find the segment, and $n+k:n$ bits to locate the bucket inside the segment.
Since the record $r$ might be inserted to bucket $b$ or bucket $b+1$, both version locks will be acquired at this time.
Before writing $r$ to the bucket, the operation will need to check duplication, by first looking at the fingerprint and then, if necessary, check the actual key. 

The inserts proceeds by check the capacity of bucket $b$ and bucket $b+1$, if any of them has free space,
the record $r$ will be placed in that bucket, set the corresponding fingerprint and membership bits, and update the version lock.
Otherwise, the thread will try to displace the keys in both buckets, as shown in Figure~\ref{fig:probe-displacement}, a key that originally belongs to bucket $b$ can be displaced to bucket $b-1$ or bucket $b+1$,
thus makes room for the new records. 
When both displacement failed, in other words, both buckets are full, instead of splitting the bucket and doubling the directory,
the thread will try to insert the record $r$ to the shared stash bucket. 
If all the above attempts failed, this indicates the segment already in a heavy load state,
and a thus segment split is necessary to consolidate the records and thus improve the search performance.
The Algorithm~\ref{alg:insert_key} and Algorithm~\ref{alg:insert_key_bucket} summaries this process. 
\todo{need to explicit mention fence and flush}

\todo{structure looks strange here}

\begin{algorithm}
	\footnotesize
	\caption{insert a record to a bucket}
	\label{alg:insert_key_bucket}
	\begin{algorithmic}[1]
		\Function{insert\_to\_bucket}{$key$, $value$, $hashed\_key$, $bucket$}
		\State $slot$ = index of first leading zero of $alloc\_bitmap$
		\State $bucket.data[slot]$ = ($key$, $value$)
		\State Persist($bucket.data[slot]$)
		\State $bucket.fingerprints[slot]$ = Fingerprint($hashed\_key$)
		\State mfence()
		\State $bucket.alloc\_bitmap[slot]$ = 1
		\State clwb($bucket.alloc\_bitmap[slot]$)
		\Comment{Persist the bitmap also write back the fingerprint, since they are in the same cacheline}
		\EndFunction
	\end{algorithmic}
\end{algorithm}

\begin{algorithm}
	\footnotesize
	\caption{insert key to hashtable}
	\label{alg:insert_key}
	\begin{algorithmic}[1]
		\Function{insert}{$key$, $value$}
		\State $hashed\_key$ = hash($key$)

		\State $fingerprint$ = Fingerprint($hashed\_key$)
		\State $bucket\_pos1$ = $hashed\_key$ \% $N$
		\Comment{current bucket}
		\State $bucket\_pos2$ = ($bucket\_pos1$ + 1) \% $N$
		\Comment{next bucket}

		\State $Buckets[bucket\_pos1].lock()$
		\State $Buckets[bucket\_pos2].lock()$
		\\
		\State $is\_duplicate$ = check duplicate $key$
		\If{$is\_duplicate$}
			\Comment{Uniqueness check}
			\State $Buckets[bucket\_pos1].unlock()$
			\State $Buckets[bucket\_pos2].unlock()$
			\State \Return true
		\EndIf
		\\
		\If{$Buckets[bucket\_pos1].count < CAPACITY$ \textbf{or}\\ $Buckets[pos_{2}].count < CAPACITY$}

		\If{$Buckets[bucket\_pos1].count \leq Buckets[bucket\_pos2].count$}
		\State $Buckets[bucket\_pos1].insert\_to\_bucket(key, value, hashed\_key)$
		\Else
		\State $Buckets[bucket\_pos2].insert\_to\_bucket(key, value, hashed\_key)$
		\EndIf
		\State \textbf{goto} \emph{InsertSuccess}
		
		\Else

		\If{Displacement\_and\_insert($bucket\_pos1, bucket\_pos2, key, value$)}
		\Comment{Conduct the displacement in two directions and try to insert the new item}
				\State \textbf{goto} \emph{InsertSuccess}
		\EndIf
		\State $stash\_pos$ = insert $key$ to stash
		\If{$stash\_pos \neq -1$}
		\State add overflowed fingerprint into corresponding bucket
		\State \textbf{goto} \emph{successInsert}
		\EndIf
		
		\State $Buckets[bucket\_pos1].unlock()$
		\State $Buckets[bucket\_pos2].unlock()$
		\State \Return false
		\Comment{Insertion Failure}
		\EndIf
		
		\BState \emph{InsertSuccess}:
		\State $Buckets[bucket\_pos1].unlock()$
		\State $Buckets[bucket\_pos2].unlock()$
		\State \Return true;
		
		\EndFunction
	\end{algorithmic}
\end{algorithm}

\subsection{Search}
The DASH design has carefully optimized read operations for fast-probing and low memory footprint, 
makes DASH extremely efficient on limited-bandwidth memories.
To query a record, a thread will first check the version lock on the directory and wait until the lock is unset,
it then checks the version lock on the two buckets, read the fingerprints, and check the keys if necessary.
The read will then finishes by checking the version lock again to make sure there's no concurrent change to the bucket.
Algorithm~\ref{alg:get_value_bucket} describes getting records from a bucket.

With the fingerprint design, read operation will not need to load and check every key, 
instead, by checking the one-byte fingerprint, it will pre-eliminate the unnecessary memory load,
this is even more beneficial in the case of variable-length key.
What's more, the lightweight version lock is co-located at the head of bucket, makes it both low-granularity and close to actual data, 
thus reduce can the cache miss and contention between threads.  

\todo{We might want to discuss more if have more space.}

\subsection{Delete}
